# Supplementary material for: TimeLogic: A Temporal Logic Benchmark for Video QA
Source: arXiv:2501.07214 source file (2025-01-13)
Supplement: Supplementary file 1 [file X_suppl.tex]

% \clearpage
\setcounter{page}{1}
\maketitlesupplementary

We organize the supplementary material as follows

\begin{itemize}
    \item Section~\ref{sec:data_details}: Dataset Details 
    \item Section~\ref{sec:add_res}: \textit{Fine-Tuning} with TLQA dataset, Zero-Shot TLQA evaluations, Additional Results
    \item Section~\ref{sec:res_dis}: Result discussion and data samples, detailed metrics
    \item Section~~\ref{sec:temp_mcq}: Templates for TLQA multiple choice questions
    \item Section~\ref{sec:application}: Potential application and benefits of framework and benchmark
    \item Section~\ref{sec:nexqa_comp}: Comparison with NExT-QA dataset
    \item Section~\ref{sec:qual}: Qualitative Analysis
\end{itemize}

\section{Dataset details} % sec 1
\label{sec:data_details}
Here, we present details for all the datasets along with their license information.
For datasets with missing annotations for all frames, we only retain the frames with annotations and use them for evaluation.

\href{https://bobbywu.com/STAR/}{\textbf{STAR}}~\cite{wu2021star_situated_reasoning}: Apache License 2.0, \url{https://github.com/csbobby/STAR/blob/main/LICENSE} \\ % \href{https://github.com/csbobby/STAR/blob/main/LICENSE}{STAR Dataset LICENSE} \\
\href{https://serre-lab.clps.brown.edu/resource/breakfast-actions-dataset/}{\textbf{Breakfast}}~\cite{Kuehne12bf}: CC BY 4.0 License, \url{http://creativecommons.org/licenses/by/4.0/} \\
\href{https://github.com/DmZhukov/CrossTask}{\textbf{CrossTask}}~\cite{Zhukov2019crosstask}: BSD 3-Clause License, \url{https://github.com/DmZhukov/CrossTask/blob/master/LICENSE}\\
\href{https://cs.stanford.edu/people/ranjaykrishna/agqa/}{\textbf{AGQA}}~\cite{GrundeMcLaughlin2021AGQA}: MIT License, \url{https://github.com/madeleinegrunde/AGQA_baselines_code/blob/main/LICENSE.md} \\

As we leverage popular datasets that are publicly available under the specified licenses above, we follow the same license for releasing the TLQA-benchmark for respective datasets. Note, we do not release datasets, we only release the TLQA-framework and benchmark. The TLQA benchmark source code is attached in the supplementary zip file, we will release the framework upon acceptance.

\section{Fine-Tuning \& Additional Results}
\label{sec:add_res}
% First, we present the results with Instruction Fine-tuning with TLQA and report zero-shot performance on our benchmark and also additional benchmarks to highlight the benefits of TLQA framework and report performance in Section~\ref{sec:tlqa_ft}. Then we present more evaluations on our benchmark in Section~\ref{sec:lita} 
We begin by presenting the results of Instruction Fine-tuning with TLQA, highlighting its zero-shot performance on both our benchmark and additional benchmarks to showcase the advantages of the TLQA framework. These results, along with a detailed performance analysis, are reported in Section~\ref{sec:tlqa_ft}. Further evaluations on our benchmark are presented in Section~\ref{sec:lita}.

\begin{table}\setlength{\tabcolsep}{2pt}
    \centering
    \resizebox{0.49\textwidth}{!}{
    \begin{tabular}{cc|ccc}
       Method & Fine- & NExTQA & \multicolumn{2}{c}{VideoMME} \\
       \cmidrule(lr){4-5}
       & Tune & & Overall & Temporal Perception \\
       \midrule
        LLaVA-OV & \redxmark & 57.2  & 43.9 & 29.1 \\
        (Ours) LLaVA-OV & \greenmark & \textbf{61.8 (+4.6)}  & \textbf{44.5} & \textbf{36.4 (+7.3)} \\ \\
        % LLaVA-OV-7B & \redxmark & 79.3 & 58.2 \\
        % LLaVA-OV-7B & \greenmark &   &  \\
    \end{tabular}
    }
    \caption{Zero-shot evaluation of our model fine-tuned on the TLQA-AGQA dataset. Comparison with LLaVA-OV: LLaVA-OneVision}
    \label{tab:tlqa_ft}
\end{table}

\subsection{Fine-tuning with TLQA dataset}
\label{sec:tlqa_ft}

As demonstrated current video models are weak at temporal understanding. To address this, we propose to leverage the annotations generated by the TLQA framework to perform Instruction Fine-tuning, enabling models to improve temporal logical understanding. For these experiments, we utilize the LLaVA-OneVision~\cite{li2024llavaOV} model, specifically LLaVA-OneVision-Qwen2-0.5b. % and fine-tune on 32K questions from TLQA derived from AGQA~\cite{GrundeMcLaughlin2021AGQA}.

% For generating training data with temporal logical operators, we generate 2000 questions for each category of temporal operator on AGQA dataset resulting in 32K QA pairs. We use this in addition to a subset of academic MCQ from LLaVA-OV training data to perform Instruction fine-tuning for 1 epoch with learning rate of 1e-6, lora rank and alpha set to 64, 16.

To create training data enriched with temporal logical operators, we generate 2,000 questions for each temporal operator category from the AGQA dataset, resulting in a total of 32K QA pairs. This dataset is combined with a subset of academic multiple-choice questions from the LLaVA-OV training data. The model is fine-tuned for one epoch with a learning rate of 1e-6, LoRA rank set to 64, and alpha set to 16.

\begin{table}\setlength{\tabcolsep}{3pt}
    \centering
    \resizebox{0.48\textwidth}{!}{
    \begin{tabular}{cc|cc}
       Temporal   & Complexity & \multicolumn{2}{c}{STAR}  \\
       \cmidrule(lr){3-4}
       Operator &    & LLaVA-OV  & \textbf{Ours} \\
       \midrule
        Eventual &  1  &  56.2 &  \textbf{74.8} \\
        Always &  2  &  56.2 & \textbf{76.6}\\
        \midrule
        Until &   3 & 44.4  & \textbf{75.4} \\
        Since &  3  &  56.6 & \textbf{75.9} \\
        Implies & 3   & 63.1  & \textbf{81.2} \\
        Before &  3  & 54.8  & \textbf{79.1}\\
        Next &  3  &  47 & \textbf{72.2} \\
        Co-Occur &  3  &  66.6 & \textbf{82.6}\\
        Disjoint & 3   & 34.2  & \textbf{76.1} \\
        \midrule
        Immediate Next & 4   & 49.9  & \textbf{72.2} \\
        Always Before &  4  & 56.9  & \textbf{79.5} \\
        Always Next & 4   & 50.7  & \textbf{79.2} \\
        Always Co-occur & 4   &  59 & \textbf{82.1} \\
        \midrule
        Strict A,B,C & 5   & 52.4  & \textbf{80} \\
        Loose A,B,C &  5  &  75 & \textbf{88.3} \\
        A always before B, C &  5  & 50.2  & \textbf{79.6} \\
        \midrule
        Mean Acc. &    &  54.6 & \textbf{78.4 (+23.8)} \\
    \end{tabular}
    }
    \caption{Evaluation on TLQA STAR benchmark with our fine-tuned model on TLQA-AGQA dataset.}
    \label{tab:tlqa_ft_star}
\end{table}

% We perform two type of evaluations for the model fine-tuned on TLQA-AGQA train data - (i) we evaluate on other splits of TLQA benchmark \ie TLQA-STAR and TLQA-CrossTask, and (ii) we also evaluate on external benchmarks like NExT-QA, VideoMME.
We conduct two types of evaluations for the model fine-tuned on TLQA-AGQA training data: (i) evaluation on other splits of the TLQA benchmark, such as TLQA-STAR and TLQA-CrossTask, and (ii) evaluation on external benchmarks, including NExT-QA and VideoMME.
% This demonstrates the benefits of leveraging the TLQA framework to generate data at any scale for instruction fine-tuning and further as shown in Tables~\ref{tab:tlqa_ft},~\ref{tab:tlqa_ft_star},~\ref{tab:tlqa_ft_ct} the performance significantly improves on all benchmarks consistency. With vast margins of gains on temporal tasks. The Zero-Shot evaluation on TLQA CrossTask in Table~\ref{tab:tlqa_ft_ct} demonstrates the improved temporal robustness with a gain of $20\%$. Further, we show detailed comparison across temporal operators and our model consistently outperforms with huge margin. 
These evaluations highlight the benefits of leveraging the TLQA framework to generate scalable data for instruction fine-tuning.  As highlighted in Tables~\ref{tab:tlqa_ft}, \ref{tab:tlqa_ft_star}, and \ref{tab:tlqa_ft_ct}, our approach consistently achieves significant performance improvements across all benchmarks, particularly on temporal tasks. For instance, zero-shot evaluation on TLQA-CrossTask benchmark demonstrates a substantial gain of $17.6\%$ in temporal robustness (see Table~\ref{tab:tlqa_ft_ct}). Similarly, on the TLQA-STAR benchmark, our model surpasses the base model with a remarkable margin of $23.8\%$. Furthermore, a detailed comparison across temporal operators shows that our model consistently outperforms LLaVA-OV by a wide margin.

On widely-used video benchmarks like NExT-QA and VideoMME, our model fine-tuned with TLQA achieves notable improvements, outperforming the base model by $4.6\%$ on NExT-QA and $7.3\%$ on the temporal perception category of VideoMME, as shown in Table~\ref{tab:tlqa_ft}.

% On other common video benchmarks like NExT-QA and VideoMME, our model fine-tuned with TLQA outperforms the base model by $4.6\%$ on NExT-QA and $7.3\%$ on the temporal perception category of VideoMME as shown in Table~\ref{tab:tlqa_ft}.

\begin{table}\setlength{\tabcolsep}{3pt}
    \centering
    \resizebox{0.48\textwidth}{!}{
    \begin{tabular}{cc|cc}
       Temporal   & Complexity & \multicolumn{2}{c}{CrossTask}  \\
       \cmidrule(lr){3-4}
       Operator &    & LLaVA-OV  & \textbf{Ours} \\
       \midrule
        Eventual &  1  & 54.2  &  \textbf{73.6} \\
        Always &  2  & -  & - \\
        \midrule
        Until &   3 & 55.3  & \textbf{71.9} \\
        Since &  3  &  - & - \\
        Implies & 3   & -  & - \\
        Before &  3  & 61.4  & \textbf{74.5}\\
        Next &  3  &  59.3 & \textbf{76.1} \\
        Co-Occur &  3  &  - & - \\
        Disjoint & 3   & 37.8  & \textbf{76} \\
        \midrule
        Immediate Next & 4   & 58.5  & \textbf{77} \\
        Always Before &  4  & 58.4  & \textbf{72.9} \\
        Always Next & 4   & 52.9  & \textbf{71.5} \\
        Always Co-occur & 4   &  - & - \\
        \midrule
        Strict A,B,C & 5   & 59.6  & \textbf{71.3} \\
        Loose A,B,C &  5  &  76.1 & \textbf{85.8} \\
        A always before B, C &  5  & 57.9  & \textbf{74.6} \\
        \midrule
        Mean Acc. &    &  57.4 & \textbf{75 (+17.6)} \\
    \end{tabular}
    }
    \caption{Zero-Shot Evaluation on TLQA CrossTask benchmark with our fine-tuned model on TLQA-AGQA dataset.}
    \label{tab:tlqa_ft_ct}
\end{table}

\subsection{More Results}
\label{sec:lita}

% Here, we benchmark on LITA~\cite{huang2025lita}, which proposes a method for temporal localization in videos to generate `timestamps'. However, it's important to note that LITA is specialized for reasoning-temporal localization task, whereas our approach offers a broader and more comprehensive solution. LITA primarily focuses on generating timestamps for temporal localization and also reasoning for that localization in videos, while our framework is designed to focus on the temporal ordering of events within the video. The performance on TLQA-S on STAR benchmark is reported in Figure~\ref{fig:lita_star}. We also present baseline scores computed by passing blank frames to the LITA model. We see that the general performance tends to drop as the temporal complexity increases.

Here, we benchmark against LITA~\cite{huang2025lita}, a method specifically designed for temporal localization in videos, which generates `timestamps' along with reasoning for those localizations. However, it is important to highlight that LITA is tailored for the reasoning-temporal localization task, whereas our framework provides a broader and more comprehensive solution. While LITA focuses on generating and reasoning about timestamps, our approach emphasizes understanding the temporal ordering of events within videos. The performance on TLQA-S on STAR benchmark is presented in Figure~\ref{fig:lita_star} with LITA-13B model. For comparison, we also include baseline scores computed by passing blank frames to the LITA model. As temporal complexity increases, we observe a general decline in performance, highlighting the challenges posed by higher levels of temporal reasoning. %Authors release only 13B model weights for LITA, hence it is not directly comparable to Table 5.

\begin{figure}%{r}{5.5cm}
% \vspace{-4em}
% \hspace{-1em}
    \centering
    \includegraphics[width=\linewidth]{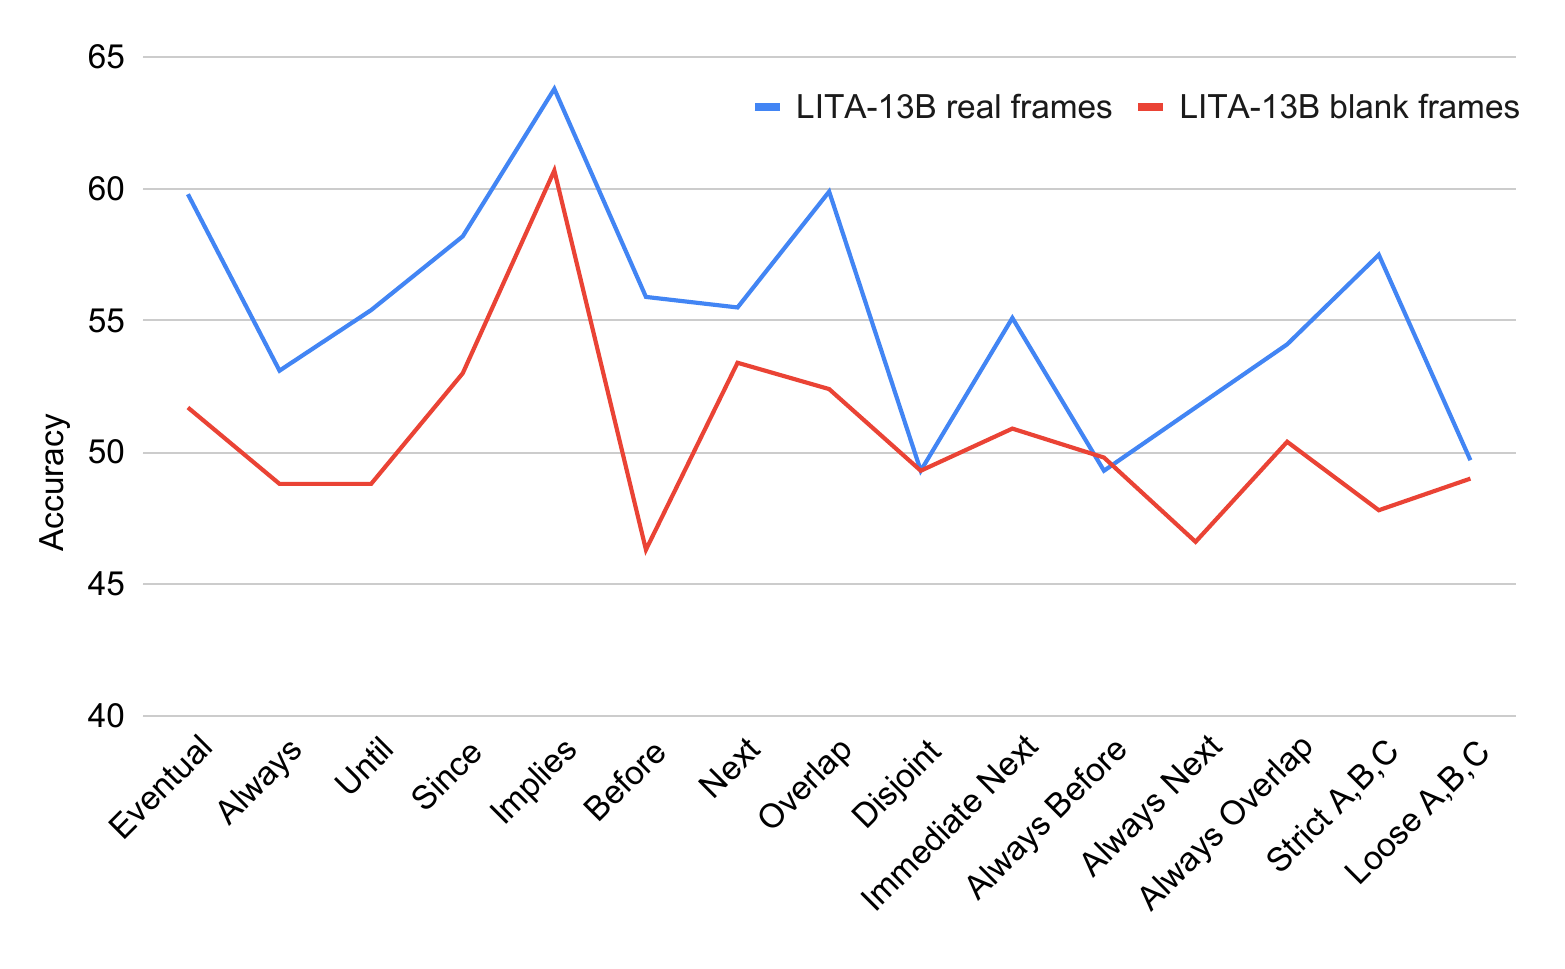}
      \caption{Zero-Shot Results on boolean TLQA-S on STAR dataset. }
      % \vspace{-1.5em}
  \label{fig:lita_star}
\end{figure}

\section{Result Discussion and Details}
\label{sec:res_dis}

% simple baseline and llovi disucss here
Here, we present text-baselines for boolean TLQA benchmark with ChatUnivi. In this experiment, we pass blank frames to the model and evaluate its performance by asking it to generate responses without relying on visual information. The results, shown in Figure~\ref{fig:bool_bs_cu}. On the Breakfast dataset, which includes structured activities such as cooking recipes, the model benefits from leveraging prior knowledge embedded in the language model, even with blank frames.
On the CrossTask benchmark, performance drops more sharply due to the lack of meaningful contextual cues in blank frames, as these tasks often require specific temporal reasoning tied to video content.

In Figure~\ref{fig:llovi_caps}, we showcase sample captions generated for the evaluation of LLoVI~\cite{zhang2023llovi}. The captions are extracted at a rate of 0.5 fps from the video using LLaVA 7B as the captioner, and the GPT-3.5-Turbo-1106 model is employed for the QA task, following the evaluation protocol outlined in LLoVI~\cite{zhang2023llovi}.
The performance in this setup heavily depends on the quality of the information captured by the captioner. It is important to note that the captioner processes only the current frame and lacks contextual knowledge of past or future frames. This independence can lead to incomplete or inaccurate descriptions, which in turn affects the overall QA performance.
% The performance here, relies heavily on the information captured by the captioner. Note that the captioner has access to only current frame and does not have knowledge about past or future making it independent thus leading to inaccurate descriptions.

\begin{figure*}
\begin{center}
    \begin{subfigure}[t]{0.48\linewidth}
\includegraphics[width=1\linewidth]{images/bool_baseline_ct_v1.pdf}
\caption{Baseline: TLQA-S on CrossTask for Boolean QA. }
\end{subfigure}%
\begin{subfigure}[t]{0.48\linewidth}
\includegraphics[width=1\linewidth]{images/bool_baseline_bf_v1.pdf}
\caption{Baseline  TLQA-S on Breakfast for Boolean QA}
\end{subfigure}%
\end{center}
\caption{ChatUnivi with real vs. blank frames comparison for boolean TLQA. We provide blank frames to ChatUniVi as a baseline to evaluate the performance on boolean TLQA benchmark. As shown the performance tends to drop as the temporal complexity increases (left-to-right). For Breakfast dataset which contains cooking receipe videos, the model is making better prediction due to better context (actions as part of the question) and LLM prior knowledge.
For CrossTask the performance drops as temporal complexity increases. %, while for Breakfast the model is able to make a guess based on LLM prior.
}
\label{fig:bool_bs_cu}
\end{figure*}

\begin{figure*}
\begin{center}
    % \begin{subfigure}[t]{\linewidth}
\includegraphics[width=0.96\textwidth]{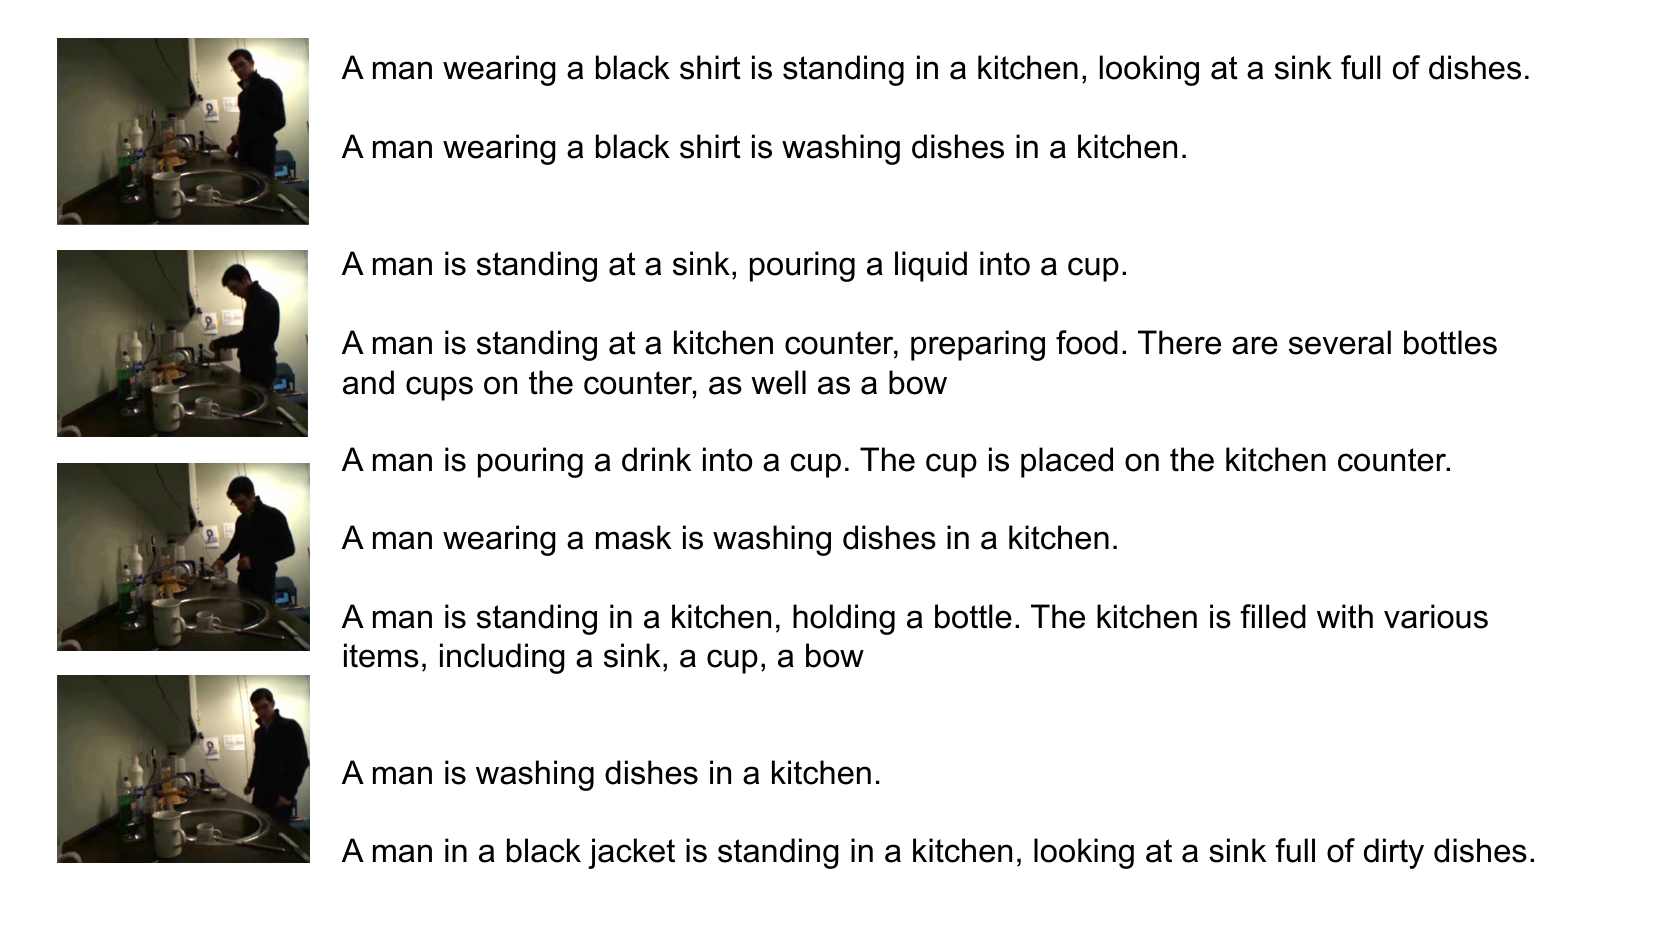}
% \caption{MC Baseline for TLQA-S on CrossTask}
% \end{subfigure}%
\end{center}
\caption{Sample captions extracted for a video making cereals from Breakfast dataset for LLoVI evaluation. The generated captions do not talk about cereals or milk indicating lower caption quality. In addition there are some hallucinations in the generated captions like washing dishes while there is no such action in the actual video.}
\label{fig:llovi_caps}
\end{figure*}

\subsection{Detailed Metrics}
Here, we present detailed metrics for the Boolean TLQA benchmark. Evaluating Boolean questions solely based on accuracy may not provide a comprehensive understanding of model performance. Therefore, in addition to accuracy, we include F1-score and $\%$ of Yes responses \ie ($\%$Yes)  to offer deeper insights into the model's capabilities. ChatUniVi~\cite{jin2023chatunivi} generally exhibits stronger performance. 
% Here, we present detailed metrics for boolean TLQA benchmark. In order to evaluate boolean questions, only relying on accuracy may not provide full insights into model performance. Hence, we present F1-score and $\%$Yes ratio along with Accuracy to provide insights into model performance. 

%%%%%%%%%%%%%%%%%%%%%%%%%%%%%%%%%%%%%%%%%%%%
% %%%% FULL table
\begin{table*} \setlength{\tabcolsep}{5pt}
  \centering
  \resizebox{\textwidth}{!}{
  \begin{tabu}{lcccccccccccccccccccccccccccc}
    \toprule
    % & & \multicolumn{4}{c}{VQAv2 Accuracy}                   \\
    % \cmidrule(r){3-6}

    Temporal & Complexity &  \multicolumn{9}{c}{STAR}  &  \multicolumn{9}{c}{Breakfast} &  \multicolumn{9}{c}{AGQA}    \\
    \cmidrule(r){3-29} 
    Operators &  Level &  \multicolumn{3}{c}{VideoLLaVA} &\multicolumn{3}{c}{VideoChatGPT} &\multicolumn{3}{c}{ChatUnivi}       &\multicolumn{3}{c}{VideoLLaVA} &\multicolumn{3}{c}{VideoChatGPT} &\multicolumn{3}{c}{ChatUnivi}      &\multicolumn{3}{c}{VideoLLaVA} &\multicolumn{3}{c}{VideoChatGPT} &\multicolumn{3}{c}{ChatUnivi}          \\

    \cmidrule(lr){3-5} \cmidrule(lr){6-8} \cmidrule(lr){9-11} \cmidrule(lr){12-14} \cmidrule(lr){15-17} \cmidrule(lr){18-20} \cmidrule(lr){21-23} \cmidrule(lr){24-26} \cmidrule(lr){27-29}
    
     & & Acc. & F1 & \%Yes     & Acc. & F1 & \%Yes     & Acc. & F1 & \%Yes    & Acc. & F1 & \%Yes        & Acc. & F1 & \%Yes     & Acc. & F1 & \%Yes &    Acc. & F1 & \%Yes    & Acc. & F1 & \%Yes      & Acc. & F1 & \%Yes     \\
       
        % &  &  &  &  &  &  &   &  &  & & &  & & &   & & &  \\      
    \midrule
    Eventual & 1    & 51.1 & 67.2  & 98.8      & 50.2  &  66.8 & 99.9      &  56.3 & 68.2  & 92.6     & 50.1  &  67.5 & 99.5       & 51.3  & 67.6  & 65.6      &   51.1&  66.9 & 97.4     & 51.5  & 67.5  & 98.7       &  50.2 &  66.8 & 99.7      &  55.2 & 68.6  & 92.2\\
    Always & 2    & 60.7 & 54.4  & 33.6      &  50.7 & 65.9  & 92.3      & 54.5  & 36.8  & 19.4     & -  &-   & -       &  - &  - &  -     &  - &-   & -     &   61.6& 50.1  & 26.5       &  46.9 & 61.3  & 86.6      & 52.6 & 26.6  & 14\\
    
    \midrule
    Until & 3    & 52.9  & 67.9  & 96      & 50.9  & 67.2  & 98.9      &  59.4 & 61.9  & 56     &  50.6 & 66.3  & 95.2       & 51.4  & 67.6  & 98.5      & 54.1  & 61.1  & 66.5     &51.3   & 66.6  & 95.3       & 50.2  &  66.7 & 99.2      &  60.3 & 64.8  & 62.6\\
    Since & 3    & 54.9 & 68.6  & 92.8      & 50.8  & 67  & 98.6      & 55.1  & 67.2  & 86.2     & -  & -  & -       & -  & -  & -      & -  & -  &   -   &    55.2& 68.5  & 91.6       & 51.2  & 67.2  & 97.9      & 54.7  & 67.1  & 87\\
    Implies & 3    & 57.3 & 68.7  & 85.9      &  62.2 & 64.6  & 56.1      & 52.6  & 65.8  &  82.1    &  - &  - & -       & -  & -  & -      & -  &-   & -     &  59.6 & 70.1  & 85       & 61.3  & 65.2  & 60.6      & 53.4  & 65.3  & 81.9 \\
    Before & 3 &  51.5  &  67.4 & 98.5     & 50.5  & 66.9  & 99.3      & 53.3  & 63.9  & 78.7     &  50.3 & 64.9  & 90.3       & 51.2  & 67.5  & 99      & 51.6  & 50.4  & 46.6     & 50.9  & 66.9  & 97.9       & 51  & 67.1  & 98.4      & 55.5  & 66.7  & 83.1\\
    Next & 3 &  52.1  &  67.8 & 98.2      & 51.1  & 67.2  & 98.3      & 56.5  & 67.5  & 83.2     & 51.5  & 67.8  & 99.6       & 52.3  & 67.6  & 96.3      &  54.8 & 64.5  & 76     & 51.3  & 67.4  & 98.9       & 50.8  & 66.8  & 97.9      &  55.6 & 67.1  & 84.8\\
    Co-occur & 3    & 51.1 & 67.4  & 99.5      & 53.4  & 58.1  & 60.5      & 58.1  & 62.7  & 61.7     &  - &  - &  -      & -  & -  &  -     & -  & -  &      & 50.2  & 66.4  & 98.3       & 54.7  & 60.5  & 64.5      & 57.6  & 62.2  & 61.9\\
    Disjoint & 3    & 51.8 & 67.5  & 97.6      & 53.1  & 65.3  & 84.2      & 46.9  & 25.6  & 20.6     & 50.9  & 67.4  & 99.9       & 50.9  & 66.7  & 96.6      & 51.8  & 39.9  & 29.3     & 51.2  & 66.9  & 97.1       & 55.6  & 66.7  & 82.9      &  49.1 & 30.3  & 22.7\\
    \midrule
    Immediate Next & 4    & 53.8 & 68.5  & 95.5    & 52.8 & 66.3  & 89.1     & 54.6 & 63.7  & 74.5    &47.6  & 60.6  &82.3         & 51.1 & 63.6  &  83.2    & 46.3 & 32.9  & 23.2    &52.3  & 66.6  & 92.1      & 52.9 &  65.6 & 86.4     & 53.4  &  66.4 & 76.8\\
    
    Always Before & 4    & 49 & 64.8  & 95.3      & 49.8  & 66.1  & 98.7      & 49.1  & 35.1  & 28.9     & 47.9  & 63.3  & 93.6       & 48.1  & 64.8  & 98.9      & 50.3  & 35.3  & 28.3     &  49 & 64.7  & 94.3       &50.7  & 66.7  & 98.2      &   50.4&  40.4 & 33.2\\
    Always Next & 4    & 49.4 & 66  & 99.4      &  49.6 & 66.2  & 98.9      & 49.6  & 49.8  & 50.9     & 47.7  & 63.8  & 95.7       & 48.6  & 64.9  & 97.3      & 48.2  & 34.7  & 30.6     & 50.5  & 66.5  & 98.2       &49.9  & 66.2  & 98.1     &  47.7 & 49.2  & 52.9\\
    Always Co-occur & 4    & 51.7 & 62.4  & 76.2      & 52.6  & 57.6  & 59.6      & 53.8  & 42.9  & 28.9     &  - &  - &   -     & -  & -  &  -     &  - & -  & -     & 56.3  & 63.1  & 68.1       & 52.2  & 56.3  & 59.1      &  56.6 & 38.5  & 20.2\\
    \midrule
    Strict A,B,C & 5    & 53  & 69.3  & 99.8      & 51.4  & 59.3  & 66.6      & 56.1  & 45.8  & 28     & 51.3  & 67.8  & 100       &  50.1 & 56.9  & 64.7      & 51.9  & 64.1  & 82.6     & 50.3  & 66.9  & 99.9       & 55  & 61.9  & 67.6      & 56.3  & 40.9  & 23.8\\
    Loose A,B,C & 5 & 51.5  &  67.2 & 97.1      & 50.8  & 66.9  & 97.6      & 52.7  & 43.6  & 33.1     & 51.1   & 67.6  & 99.8       & 49.6  & 65.8  & 96.2      & 50.8  & 49.6  & 46.5     & 50.6  & 66.4  & 96.7       &  50.4 & 66.2  & 96.5      &  55.2 & 44.2  &  34.6\\
    A always before B,C & 5    & 51.2  & 67.6  & 99.6      & 50.9  & 65.4  & 90.9      & 55.1  &  44 &  29.2    & 51.2  & 67.7  & 100        &  50.1 & 65.4  & 92.9      &  52.9 & 58.3  & 61.9     & 51.1  & 67.4  &99.4        &  50.5 & 65.2  & 91.2      & 56.6  & 43.1  & 25.9\\

    % Mean Acc \\
    \bottomrule
  \end{tabu}
  }
  \caption{Detailed Metrics for zero-shot evaluation on boolean QA TLQA-S across STAR, Breakfast and AGQA. }
  \label{tab:supp_tlr_small}
  % \vspace{-0.2in}
\end{table*}

\section{Templates for MCQ}
\label{sec:temp_mcq}
Here, we present the template questions for multiple-choice TLQA benchmark in Table~\ref{tab:templates_what_format}. Each multiple-choice question has 4 options, the model has to pick the correct answer choice.

\begin{table*}\setlength{\tabcolsep}{5pt}
  \centering
  \resizebox{\textwidth}{!}{
  \begin{tabu}{lcc}
    \toprule
      \textbf{ Temporal Operators} & \textbf{Complexity} &  \textbf{Template Questions }  \\
       % Operators &  &   \\      
    \midrule
    Eventual & 1 &   What does the <person> do in this video ? \\
    Always & 2 & What action does the <person> do throughout the video ? \\ % $<{action}\_0>$
    Until & 3 & What did the <person> do until <action> ? \\
    Since & 3 & What has been the <person> doing since they <action> ? \\
    Implies & 3 & \makecell{While the <person> is <action>, what does \\this imply about <person> action ?}  \\
    %Overlap &  & &   &  &   &   & \\      
    Before &  3 &  What did the <person> do before <action> ? \\
    Next & 3 & What did the <person>  do after <action> ? \\
    Co-Occur & 3 & What does the <person> do when <action>? \\
    % Immediate Before &  4 &  \\
    Disjoint & 3 & Which action by the <person> does not overlap with <action> ? \\
    Immediate Next & 4  & What did the <person> do immediately after <action> ?  \\
    Always Before & 4 & What did the <person> do always before <action> ? \\
    Always Next & 4 & What did the <person> do always after <action> ? \\
    Always Co-Occur & 4 &  Which action always co-occurs with <action> ? \\
    \midrule
     \multicolumn{3}{c}{\textbf{Compounding}} \\
    \midrule 
    Strict A,B,C & 5 &  \makecell{ Which action always occurs before <person> <action> which \\ in turn always occurs before <person> <action> ? }\\
    
    Loose A,B,C &  5&  \makecell{Which action occurs before <person> <action> which  \\ in turn occurs before <person> <action> ?}\\
    A always before B,C & 5 &  \makecell{Which action always occurs before <person> <action> \\ and <person> <action> ?} \\
    \bottomrule
  \end{tabu}
  }
  \caption{Illustration of multiple choice template questions for each category of TLQA benchmark.}
  \label{tab:templates_what_format}
  % \vspace{-0.2in}
\end{table*}

\section{Potential Applications and Benefits}
\label{sec:application}
We would like to highlight that the dataset generated with our framework serves as a comprehensive testbed for evaluating temporal understanding capabilities in videos, offering a valuable resource for advancing research in this area. One of the key advantages of our framework is its independence from external models such as ChatGPT or human involvement, making it highly versatile and applicable to any dataset with temporal annotations.%As our framework does not rely on external models like Chat-GPT/human involvement it can be applied to any dataset with temporal annotations.
% Moreover, we see potential for future extensions, as our framework is designed to be both generic and flexible. It can be easily adapted to work with other types of temporal annotations, such as temporal object-relations and temporal action-object-relations. Additionally, it could be extended to include dense caption annotations alongside temporal data, further enhancing its applicability. Furthermore, there is potential for the generated annotations to be used for Instruction fine-tuning as presented in Section~\ref{sec:tlqa_ft}. 
Our framework is designed to be both generic and flexible, with significant potential for future extensions. It can be easily adapted to incorporate other types of temporal annotations, such as temporal object-relations and temporal action-object-relations. Additionally, it could be extended to include dense caption annotations alongside temporal data, further broadening its utility.

\begin{figure*}
    \centering
    \includegraphics[width=\linewidth]{images/qual_tlqa_i0.png}
    \caption{Qualitative comparison for the temporal operator - Loose A,B,C \ie A occurs before B, B occurs before C. VL: VideoLLaVA, VCG: VideoChatGPT, CV: ChatUniVi}
    \label{fig:qual_i0}
\end{figure*}

\begin{figure*}
    \centering
    \includegraphics[width=\linewidth]{images/qual_tlqa_i1.png}
    \caption{Qualitative comparison for the temporal operator - always before. VL: VideoLLaVA, VCG: VideoChatGPT, CV: ChatUniVi }
    \label{fig:qual_i1}
\end{figure*}

\begin{figure*}
    \centering
    \includegraphics[width=\linewidth]{images/qual_tlqa_i2.png}
    \caption{Qualitative comparison for the temporal operator - before. VL: VideoLLaVA, VCG: VideoChatGPT, CV: ChatUniVi }
    \label{fig:qual_i2}
\end{figure*}

Furthermore, the generated annotations can be utilized for Instruction Fine-Tuning, as highlighted in Section~\ref{sec:tlqa_ft}, enabling models to develop a better understanding of temporal relationships and significantly improving their performance on video temporal tasks.
% Moreover, the generated annotations offer the potential to be leveraged for Instruction Fine-Tuning, as demonstrated in Section~\ref{sec:tlqa_ft}, enabling models to gain a better temporal understanding and enhancing their overall performance on complex video tasks.

% \section{Further Benchmarking}
% \label{sec:more}

\section{Detailed Comparison with NExT-QA}
\label{sec:nexqa_comp}
% We provide detailed comparison w.r.t NExT-QA dataset in Table~\ref{tab:nextqa_comp}.
We provide a detailed comparison of the NExT-QA dataset in Table~\ref{tab:nextqa_comp}, focusing on the number of questions categorized by temporal operators such as "Immediately/Right After" and "Right Before" across NExT-QA (Multiple Choice), NExT-OE (Open-Ended), and our benchmark.

\begin{table}\setlength{\tabcolsep}{2pt}
    \centering
    \begin{tabular}{c|ccc}
       Temporal  & NExT-QA 	&NExT-OE &	TLQA-S   \\
       Operator &  MCQ & Open-ended & (Ours) \\
       \midrule
        Immediately/Right after	 &  7 & 4 & 8000 \\
        Right before	  & 3 & 3  & 8000 \\
    \end{tabular}
    \caption{Comparison of number of questions in NExT-QA/OE in test/val split and our benchmark (TLQA-S) for immediately/right before and after}
    \label{tab:nextqa_comp}
\end{table}

\begin{figure*}
    \centering
    \includegraphics[width=\linewidth]{images/qual_tlqa_i3.png}
    \caption{Qualitative comparison for the temporal operator - immediately after. VL: VideoLLaVA, VCG: VideoChatGPT, CV: ChatUniVi }
    \label{fig:qual_i3}
\end{figure*}

\begin{figure*}
    \centering
    \includegraphics[width=\linewidth]{images/qual_tlqa_i4.png}
    \caption{Qualitative comparison for the temporal operator - always before. VL: VideoLLaVA, VCG: VideoChatGPT, CV: ChatUniVi }
    \label{fig:qual_i4}
\end{figure*}

\section{Qualitative Analysis}
\label{sec:qual}
Here, we present qualitative analysis from the TLQA benchmark.

Figure~\ref{fig:qual_i0} highlights the discrepancy between model predictions and the ground truth answer, showcasing the challenges models face in accurately reasoning about complex temporal relationships. Despite the visual cues provided, all models fail to correctly interpret the temporal sequence, indicating a need for improved temporal reasoning capabilities in such scenarios. In Figure~\ref{fig:qual_i1} a qualitative comparison for the temporal operator "Always Before," which evaluates whether event A (adding kimchi) always occurs before event B (pouring sesame oil) is shown. The query asks: "Did the person add kimchi always before pouring sesame oil?". The figure highlights failure of all evaluated models in capturing consistent temporal relationships between actions.

We then present qualitative comparison for temporal operator "Before", which assesses whether event A (adding kimchi) occurs before event B (pouring sesame oil). The query posed is: "Did the person add kimchi before pouring sesame oil?" in Figure~\ref{fig:qual_i2}.
The results show that VL and CV correctly predict "Yes," aligning with the ground truth answer, while VCG fails to identify the correct temporal sequence, predicting "No." This highlights the varying capabilities of the models in reasoning about temporal relationships. 

For the given video in Figure~\ref{fig:qual_i3}, we evaluates the temporal operator "Immediately After," which examines whether event A (packing cucumbers in a jar) occurs immediately after event B (pouring vinegar). The query is: "Did the person pack cucumbers in the jar immediately after pouring vinegar?". All three models successfully identify the correct temporal relationship and align with the ground truth answer.

Figure~\ref{fig:qual_i4} examines harder case scenario for the temporal operator "Always Before," which evaluates whether event A (assembling the shelf) consistently occurs before event B (sanding the shelf). The query posed is: "Did the person assemble the shelf always before sanding the shelf?"
In this scenario, sanding occurs twice—once immediately after assembling the shelf and again at the end of the video. This dual occurrence makes the "Always Before" condition more challenging to evaluate, as it requires the model to recognize that sanding does not consistently follow assembly throughout the entire sequence..
Both VL and VCG incorrectly predict "Yes," failing to account for the second instance of sanding, while CV correctly identifies the answer as "No," aligning with the ground truth. This example highlights the complexity of temporal operators like "Always Before" in cases where the same action occurs multiple times at different points in the sequence.

% \noindent \textbf{\textcolor{red}{Annotation Discussion}}
\noindent \textbf{Annotation Discussion}
The most common problem in temporal annotation is annotator disagreement w.r.t temporal boundaries. This problem only arises in our case for temporally overlapping actions only, which only happen in STAR and AGQA datasets.
This can affect temporal categories with more than one action. For instance, in co-occur where if Action A annotation ends late and Action B annotation starts earlier, actions A and B would be considered co-occurring. To reduce these errors, we have already excluded cases from the TLQA benchmark that have overlap/gap of less than a 20\% threshold.

For the Breakfast and CrossTask datasets, they allow only single temporal annotation for every frame in the video. So for these datasets, there cannot be any unintentional gaps/overlaps. We will clarify this in the paper.

Semantic annotation errors are beyond the scope of this work. We assume if they arise they would be very rare, since these datasets have been widely used and have been thoroughly checked and vetted by the community. %In case of those errors the responsibility relies with original dataset creators and they would be responsible for fixing the errors. In that case, we would adapt the benchmark with updated annotations.

% \section{Rationale}
% \label{sec:rationale}
% % 
% Having the supplementary compiled together with the main paper means that:
% % 
% \begin{itemize}
% \item The supplementary can back-reference sections of the main paper, for example, we can refer to \cref{sec:intro};
% \item The main paper can forward reference sub-sections within the supplementary explicitly (e.g. referring to a particular experiment); 
% \item When submitted to arXiv, the supplementary will already included at the end of the paper.
% \end{itemize}
% % 
% To split the supplementary pages from the main paper, you can use \href{https://support.apple.com/en-ca/guide/preview/prvw11793/mac#:~:text=Delete%20a%20page%20from%20a,or%20choose%20Edit%20%3E%20Delete).}{Preview (on macOS)}, \href{https://www.adobe.com/acrobat/how-to/delete-pages-from-pdf.html#:~:text=Choose%20%E2%80%9CTools%E2%80%9D%20%3E%20%E2%80%9COrganize,or%20pages%20from%20the%20file.}{Adobe Acrobat} (on all OSs), as well as \href{https://superuser.com/questions/517986/is-it-possible-to-delete-some-pages-of-a-pdf-document}{command line tools}.
